# Supplementary material for: EXOTIC: An Exact, Optimistic, Tree-Based Algorithm for Min-Max Optimization
Source: arXiv:2508.12479 source file (2026-05-23)
Supplement: Supplementary file 1 [file Parameters_AGP_GDA.tex]

First, we recall the AGP algorithm from \cite{xu2023unified}, of which GDA is a special case. Next, we state the parameter choices of AGP and GDA algorithm for every experiment in Section \ref{sec: Numerics}. 

{\color{blue}
The AGP algorithm is a gradient-based algorithm, proposed in \cite{xu2023unified}, to solve \(\min_{\mbf{x}\in X}\max_{\mbf{y}\in Y} f(\mbf{x},\mbf{y})\). In particular, for every \(t\in [1:T],\) it unfolds as follows:
\begin{align*}
\mbf{x}_{t+1} &= \Pi_{{X}}\!\left(\mbf{x}_t - \frac{\nabla_x f(\mbf{x}_t,\mbf{y}_t)}{\beta(t{+}1)} - \frac{b(t{+}1)}{\beta(t{+}1)}\,\mbf{x}_t\right),\\
y_{t+1} &= \Pi_{\mathcal{Y}}\!\left(\mbf{y}_t + \frac{\nabla_y f(\mbf{x}_t,\mbf{y}_t)}{\gamma(t{+}1)} - \frac{c(t{+}1)}{\gamma(t{+}1)}\,\mbf{y}_t\right),
\end{align*}
where $\Pi_X, \Pi_Y$ denote the projection operator on the sets \(X, Y\), respectively. Additionally, $b(\cdot)$, $c(\cdot)$, $\gamma(\cdot)$, $\beta(\cdot)$ are step-size schedules. Note that GDA is an special case of AGP with $b(\cdot) = 0$ and $c(\cdot) = 0$. 

Following \cite{xu2023unified}, we choose the step-size schedules according to the Lipschitz constants of the partial gradients of \(f\). 
We describe the exact schedules used by both the algorithms for each of the problems below. 

\subsection{Parameters of AGP and GDA for Hand-crafted Example in Section \ref{subsec:hand_crafted_example}}\label{ref:app_AGP_GDA_parameters_TE2}
For AGP implementation, for every \(t\in [1:T],\) we use    
\begin{align*}
    b(t) &= \frac{0.95}{\bar\eta}\,t^{-1/4}, \\
    c(t) &= 0,
 \\ 
\beta(t) &= 1/\bar\eta, \\ 
\gamma(t) &= \bar\nu+\bar\gamma(t), \\ 
\bar\gamma(t) &= \bar\eta d_y + \frac{16 d_y}{\bar\eta\,b(t{+}1)^2}\max\!\left(\frac{0.1128}{\bar\eta}\cdot\frac{6 d_y^{3/2}+\bar\nu-\bar\eta d_y}{d_y},\,2\right) - 2\bar\nu,
\end{align*}
where we set $\bar\eta=10$ and $\bar\nu=0.1$. 
% are obtained after running a sweep over the set $\{10^{-2},10^{-1},1,10,10^2\}$. 
For GDA, we set
\begin{align*}
\beta(t)&=\frac{1}{0.9}(t{+}1)^{0.6}, \\
\gamma(t)&=\frac{1}{0.6}(t{+}1)^{0.9},\\
b(t) &= 0, \\ 
c(t) &= 0. 
\end{align*}

\subsection{Parameters of AGP and GDA for problems in Section \ref{ssec:BenchmarkSIPAMPL}}
For GDA implementation, we set \(\beta(t) = 600\,(t{+}1)^{0.9}\) and \(\gamma(t) = 900\,(t{+}1)^{0.6}\) for all benchmark problems considered in Section~\ref{ssec:BenchmarkSIPAMPL}.

For AGP implementation, we set 
\begin{align*}
    b(t) &= \frac{0.95}{\bar\eta}\,t^{-1/4}, \\
    c(t) &= 0,\\
    \beta(t) &= \frac{1}{\bar{\eta}},    \\
    \gamma(t) &= \bar\eta L_{21}^2 + \frac{16\tau L_{21}^2}{\bar\eta\,b(t{+}1)^2} - \bar\nu, 
\end{align*}
where 
\begin{align*}
    \tau &= \max\!\left(\frac{0.1128}{\bar\eta}\cdot\frac{6L_{21}^3+\bar\nu-\bar\eta L_{21}^2}{L_{21}^2},\,2\right),
\end{align*}
and \(\bar{\eta}, \bar{\nu}\) are hyper-parameters to be set for each problem separately. Moreover, for every \(\mbf{x}\in X\) and \(\mbf{y}\in Y\), let \(L_{11}\) be the Lipschitz constant of \(\nabla_{\mbf{x}} f(\cdot,\mbf{y})\), \(L_{21}\) be the Lipschitz constant of \(\nabla_{\mbf{x}} f(\mbf{x},\cdot)\), \(L_{22}\) be the Lipschitz constant of \(\nabla_{\mbf{y}} f(\mbf{x},\cdot)\), and \(L_{12}\) be the Lipschitz constant of \(\nabla_{\mbf{y}} f(\cdot,\mbf{y})\).

Next, we provide the hyper-parameters for each problem in the following table:  
% \subsubsection{Parameters for \texttt{hettich4 \cite{hettich_1979}}}\label{app:AGP_GDA_hettich4}
\begin{center}
\begin{tabular}{@{}lccc@{}}
\toprule
Quantity & \texttt{hettich4 \cite{hettich_1979}} & \texttt{hettich5 \cite{hettich_1979}} & \texttt{leon10 \cite{LEON200078}} \\
\midrule
$T$ & $300000$ & $10000$ & $10000$ \\
$L_{11},L_{12},L_{21},L_{22}$ & $100$ & $100$ & \(10\)\\
$\bar\eta$ & $0.1$ & $0.1$ & \(0.01\) \\
$\bar\nu$ & $0.1$ & $0.1$ & \(0.01\)
% \\
% $\beta(t)$ & $1/\bar\eta$ & $600\,(t{+}1)^{0.9}$ \\
% $\gamma(t)$ & $\bar\nu+\bar\gamma(t)$ & $900\,(t{+}1)^{0.6}$ \\
% $b(t)$, $c(t)$ & $q(t)$, $0$ & $0$, $0$ 
\\
\bottomrule
\end{tabular}\label{tab:table}
\end{center}

% \subsubsection{\texttt{hettich5 \cite{hettich_1979}, SIPAMPL Database}}\label{app:AGP_GDA_hettich5}
% \begin{center}
% \begin{tabular}{@{}lcc@{}}
% \toprule
% Quantity & AGP & GDA \\
% \midrule
% $T$ & $100000$ & $10000$ \\
% $L_{11},L_{12},L_{21},L_{22}$ & $100$ & $100$ \\
% $\bar\eta$ & $0.1$ & $10$ \\
% $\bar\nu$ & $0.1$ & $0.1$ \\
% $\beta(t)$ & $1/\bar\eta$ & $600\,(t{+}1)^{0.9}$ \\
% $\gamma(t)$ & $\bar\nu+\bar\gamma(t)$ & $900\,(t{+}1)^{0.6}$ \\
% $b(t)$, $c(t)$ & $q(t)$, $0$ & $0$, $0$ \\
% \bottomrule
% \end{tabular}
% \end{center}

% \subsubsection{\texttt{leon10 \cite{LEON200078}}}\label{app:AGP_GDA_leon10}
% \vspace{10pt}
% \begin{center}
% \begin{tabular}{@{}lcc@{}}
% \toprule
% Quantity & AGP & GDA \\
% \midrule
% $T$ & $100000$ & $100$ \\
% $L_{11},L_{12},L_{21},L_{22}$ & $10$ & $10$ \\
% $\bar\eta$ & $0.01$ & $10$ \\
% $\bar\nu$ & $0.01$ & $0.1$ \\
% $\beta(t)$ & $1/\bar\eta$ & $0.6\,(t{+}1)^{0.9}$ \\
% $\gamma(t)$ & $\bar\nu+\bar\gamma(t)$ & $0.9\,(t{+}1)^{0.6}$ \\
% $b(t)$, $c(t)$ & $q(t)$, $0$ & $0$, $0$ \\
% \bottomrule
% \end{tabular}
% \end{center}

\subsection{Security strategy computation}
The parameters used for AGP in Section \ref{ssec:MultiplayerGames} are the same as those in Section \ref{ref:app_AGP_GDA_parameters_TE2}. For GDA, a slightly different set of schedules was selected post running a hyperparameter sweep.  
\begin{align*}
\beta(t)&=\frac{1}{0.6}(t{+}1)^{0.98},    \\
\gamma(t)&=\frac{1}{0.9}(t{+}1)^{0.56}, \\ 
b(t) &= 0, \\ 
c(t) &= 0. 
\end{align*}

}
