# Supplementary material for: EXOTIC: An Exact, Optimistic, Tree-Based Algorithm for Min-Max Optimization
Source: arXiv:2508.12479 source file (2026-05-23)
Supplement: Supplementary file 2 [file StroquOOL_Algo.tex]

Next, we present our solution approach for solving the reformulated optimization problem \eqref{eq: SolveReformulation}, namely
\[
\max_{\mbf{w}\in \setSOO}\outerObj(\mbf{w}).
\]

{\color{blue}
Our algorithmic approach builds on the StroquOOL algorithm of \cite{bartlett2019simple}, which was originally designed for global optimization with access to noisy evaluations of a non-convex objective, where the noise is assumed to be zero-mean and handled via concentration arguments. In contrast, in our setting the objective \(G(\mbf{w})\) is itself defined as the optimal value of a convex optimization problem and can only be evaluated approximately via a finite-time solver, resulting in deterministic, biased, and iteration-dependent  estimation error. Accordingly, our method consists of two components: (i) an \emph{outer global optimization procedure} over \(\mbf{w}\in \setSOO\), which follows the StroquOOL hierarchical partitioning strategy, and (ii) an \emph{inner evaluation procedure} that approximates \(\outerObj(\mbf{w})\) by solving a convex optimization problem up to a prescribed accuracy, thereby inducing a structured inexact oracle. We introduce the algorithmic pipeline here for completeness.
}

To introduce the algorithm, we need to define a \emph{hierarchical partitioning} of the set \(\setSOO\) (recall the definition of \(\setSOO\) from Proposition \ref{prop: ProblemReformulate}). This partitioning is constructed recursively and is parameterized by an integer \(\kTree\in \N\). We denote the initial (trivial) partition as \(\setSOO_0 = \setSOO\). 
For any \(h \in \mathbb{N}\), the \(h^{\text{th}}\) partition, denoted by \(\setSOO_h\), divides the set \(\setSOO\) into \(\kTree^h\) disjoint subsets. For any \(i \in [\kTree^h]\), we denote the \(i^{\text{th}}\) subset at level \(h\) by \(\setSOO_{h,i}\). This partitioning is hierarchical in the sense that for each \(i\in [\kTree^h], h\in \N,\) each set \(\setSOO_{h,i}\) is further partitioned into \(\kTree\) disjoint subsets to obtain the partition \(\setSOO_{h+1}\). 

Throughout the remainder of the paper, we represent this hierarchical structure as a \(\kTree\)-ary tree, denoted by \(\tree\). At any depth \(h\in \N,\) the tree has \(\kTree^{h}\) nodes. For any \(i\in [\kTree^h], h\in \N,\) the node \((h,i)\) of the tree is denoted by \(\tree_{h,i}\), which is characterized by the tuple \((\varSOO_{h,i}, \estSOO_{h,i}, \optSOO_{h,i}, \num_{h,i})\) such that 
\begin{enumerate}[labelwidth=*,align=left, widest=iii, leftmargin=*]
    \item[(i)] \(\varSOO_{h,i}\in \setSOO_{h,i}\), referred to as the \emph{node center}, is a representative point such that \(\outerObj(\varSOO_{h,i})\) is used as an estimate of the function \(\outerObj\) on the set \(\setSOO_{h,i}\). 
    \item[(ii)] \(\estSOO_{h,i}\), referred to as the \emph{approximate node value}, is an approximation of \(\outerObj(\varSOO_{h,i})\) that is provided by the optimization solver \(\OPT\).
    \item[(iii)] \(\optSOO_{h,i}\), referred to as the \emph{node initializer}, is the initializer for the optimization solver \(\OPT\) that is used to evaluate \(\outerObj(\varSOO_{h,i})\). 
    \item[(iv)] \(\num_{h,i}\) is the number of iterations of the optimization solver \(\OPT\) required to obtain the approximate node value \(\estSOO_{h,i}\). 
\end{enumerate}

The resulting procedure consists of three phases:

{\paragraph{Phase I: Initialization Phase} We initialize the tree \(\tree\) with the root node and its \(\kTree\) child nodes at depth \(h=1\), labeled \(\{(1, i)\}_{i \in [\kTree]}\). For each child node \((1, i)\), we evaluate the optimization solver \(\OPT\) for \(\hmax\) iterations to compute its approximate node value \(\estSOO_{1, i}\). 

\paragraph{Phase II: Tree-expansion Phase} After the initialization phase, the tree \(\tree\) is then expanded sequentially as described below (refer \textsf{lines 2-11} in Algorithm \ref{alg: Algorithm_ComputingSol}). At each depth \(h\in [\hmax]\), we expand \(\lfloor \hmax / h \rfloor\) leaf nodes (i.e., a node without children) by adding \(\kTree\) child nodes to these nodes at depth \(h+1\). For each expansion step indexed by \(m \in [\lfloor \hmax / h \rfloor]\), we select a leaf node \((h, i)\)  that 
\begin{enumerate}[labelwidth=*,align=left, widest=iii, leftmargin=*]    
\item[(i)] has been evaluated at least \(\lfloor \hmax / (h m) \rfloor\) times by the solver \(\OPT\), and
\item[(ii)] has the highest approximate node value amongst remaining leaf nodes at depth \(h\) (refer \textsf{line 4} in Algorithm \ref{alg: Algorithm_ComputingSol}). 
\end{enumerate}

This node is then expanded by adding \(\kTree\) children at depth \(h+1\). Each new child node \((h+1, j)\) is evaluated using \(\OPT\) for \(\lfloor \hmax / (h m) \rfloor\) steps to compute its approximate node value \(\estSOO_{h+1, j}\) (refer \textsf{lines 5-9} in Algorithm \ref{alg: Algorithm_ComputingSol}).

\paragraph{Phase III: Re-evaluation Phase} Once the tree has been expanded up to depth \(\hmax\), we enter a \emph{re-evaluation phase} (refer to \textsf{Lines 12–14} in Algorithm~\ref{alg: Algorithm_ComputingSol}), which is introduced to ensure that the optimal tree node is not missed since different nodes are evaluated different number of times by the optimization solver \(\OPT\). Let \(P = \left[\left\lfloor \log(\hmax) \right\rfloor\right]\) denote the set of re-evaluation indices. For each \(p \in P\), we select a node \((h_p, i_p)\) that has been evaluated at least \(2^p\) times and has the highest approximate node value \(\estSOO_{h_p, i_p}\) among such nodes. We then re-evaluate each selected node \((h_p, i_p)\) through \(\OPT\) for \(\lfloor \hmax / 2 \rfloor\) steps to find its final approximate node value.

Finally, we return the node among \(\{(h_p, i_p)\}_{p \in P}\) that achieves the highest approximate value \(\estSOO_{h_p, i_p}\) (refer to \textsf{Lines 15–16} in Algorithm~\ref{alg: Algorithm_ComputingSol}).
A detailed description of the above procedure is presented in Algorithm \ref{alg: Algorithm_ComputingSol}.}
\begin{algorithm}[h!]
\caption{{\textbf{EXOTIC:} \textbf{EX}act, \textbf{O}ptimistic, \textbf{T}ree-based Algor\textbf{I}thm for \textbf{C}onvex--Non-concave (and Non-convex--Concave) {Minimax} Optimization }}
\begin{algorithmic}[1]
\STATE \textbf{Initialize:} 
\begin{itemize}
% \item The function \(\innerObj\) (refer \eqref{eq:CSIP_to_max_min}) and the set-valued mapping \(\setmap(\cdot)\) (refer \eqref{eq: g_equation}). 
  \item The total number of iterations of the optimization solver to \(\iter\) and the maximum depth of the tree \(\hmax.\)
  \item For any \(i\in [\kTree^h], h\in [\hmax],\) set representative points \(\varSOO_{h,i}\in \setSOO_{h,i}\) and \(\optSOO_{h,i} \in \setmap(\varSOO_{h,i})\)
   \item Tree \(\tree\) with root node \(\{(0,1) = \varSOO_{0,1}, \estSOO_{0,1} \leftarrow 0, \optSOO_{0,1}\}\). 
  \item {\color{blue}Append the nodes \(\{(1,i) = (\varSOO_{1,i}, \estSOO_{1,i} \leftarrow F(\OPT(\varSOO_{1,i}, \optSOO_{h,i}, \hmax), \varSOO_{1,i}), \optSOO_{h,i})\}_{i \in [\kTree]}\) as children of \((0,1)\) in \(\tree\).}
  \item Set \(\{\num_{1,i} \leftarrow \hmax\}_{i \in [\kTree]}\).
\end{itemize}

{\color{blue}\%\textsf{Tree-expansion phase}}
% \ENSURE Estimated optimum \(\hat{y}\)
\FOR{\(h = 1\) to \(\hmax\)}
    \FOR{\(m = 1\) to \(\lfloor \hmax / h \rfloor\)}
        \STATE Select a leaf node \((h, \bar{i})\) such that  \(
            \bar{i} \in \underset{(h,i)\in \tree_{\text{leaf}} ~ \text{s.t.} ~  \num_{h,i} \geq \lfloor \hmax/(hm)\rfloor} {\arg\max} ~ \estSOO_{h, i},
        \)
        where \(\tree_{\text{leaf}}\) denotes the set of leaf nodes of \(\tree\)
        \STATE Update \(\tree\) by adding \(\kTree\) child nodes \(\{ (h+1, j) = (\varSOO_{h+1, j}, \estSOO_{h+1, j}\leftarrow 0, \optSOO_{h+1, j})\}_{j\in [\kTree]}\) to the node \((h,\bar{i})\)
        \FOR{\(j = 1\) to \(j = \kTree\)}  
            % \STATE \(\tilde{\mbf{x}}_{h+1,j} \leftarrow \textsf{OPT}(\varSOO_{(h+1,j)}, K_{m,h}, \tilde{\mbf{x}}_{h+1,j})\)
            \STATE {\color{blue}Set \(\estSOO_{h+1, j} \leftarrow F(\OPT(\varSOO_{h+1,j},  \optSOO_{h+1,j}, \lfloor \hmax/(hm) \rfloor),\varSOO_{h+1,j} )\)}
            \STATE Set \(\num_{h+1,j} \leftarrow \lfloor \hmax/(hm) \rfloor \)
        \ENDFOR
    \ENDFOR
\ENDFOR

{\color{blue}\%\textsf{Re-evaluation phase}}

\FOR{\(p = 0\) to \(\lfloor \log_2(\hmax) \rfloor\)}
    \STATE \((h_p, i_p) \leftarrow \underset{(h,i)\in \tree :~ \num_{h,i} \geq 2^p}{\arg\max} \estSOO_{h,i},\) 
    \STATE {\color{blue}\(\estSOO_{h_p, i_p} \leftarrow F(\OPT(\varSOO_{h_p,i_p},  \optSOO_{h_p,i_p}, \lfloor \hmax/2 \rfloor), \varSOO_{h_p,i_p})\)}
\ENDFOR
\STATE Set \(\pOut \leftarrow \underset{p\in [\lfloor\log_2(\hmax)\rfloor]}{\arg\max} ~ \estSOO_{h_p, i_p}\), \(\returnSol \leftarrow \varSOO_{h_{\pOut}, i_{\pOut}},\) and \(\returnVal \leftarrow \estSOO_{h_{\pOut}, i_{\pOut}}\)
\RETURN \(\returnVal, \returnSol\)
\end{algorithmic}\label{alg: Algorithm_ComputingSol}
\end{algorithm}

\begin{algorithm}[h!]
\caption{\textbf{EXOTIC:} Tree-based outer search with convex inner evaluation}
\label{alg: Algorithm_ComputingSol}
\begin{algorithmic}[1]

\STATE \textbf{Input:} total solver budget $\iter$, maximum tree depth $\hmax$
\STATE \textbf{Initialize:}
\begin{itemize}
    \item Objective {\color{blue}$G(\mbf{w}) = \min_{{\mbf{x}}\in X}F({\mbf{x}},\mbf{w})$ over $\mbf{w}\in\setSOO$}
    \item Hierarchical partition $\{\setSOO_{h,i}\}_{h\in[\hmax],\,i\in[\kTree^h]}$ of $\setSOO$
    \item Representative points $\varSOO_{h,i}\in\setSOO_{h,i}$ and {\color{blue}initializers $\optSOO_{h,i}\in X$}
    \item Tree $\tree$ with root node $(0,1)$
\end{itemize}

\STATE \textbf{Define evaluation rule:} for any node $(h,i)$ and budget $s$, {\color{blue}\(
\estSOO_{h,i}(s) := F(\OPT(\varSOO_{h,i},\optSOO_{h,i},s), \varSOO_{h,i}).\)}

\STATE \textbf{Initial expansion:} append children $\{(1,i)\}_{i\in[\kTree]}$ to the root and set
\[
\estSOO_{1,i} \leftarrow \estSOO_{1,i}(\hmax), \qquad
\num_{1,i} \leftarrow \hmax, \qquad i\in[\kTree].
\]

\vspace{0.4em}
\STATE \textcolor{blue}{\%\textsf{Outer tree-expansion phase}}
\FOR{$h=1$ to $\hmax$}
    \FOR{$m=1$ to $\lfloor \hmax/h \rfloor$}
        \STATE Select a leaf node $(h,\bar{i})$ such that
        \[
        \bar{i}\in
        \arg\max_{(h,i)\in \tree_{\mathrm{leaf}} \,:\, \num_{h,i}\ge \lfloor \hmax/(hm)\rfloor}
        \estSOO_{h,i}.
        \]
        \STATE Expand $(h,\bar{i})$ by adding its $\kTree$ children
        $\{(h+1,j)\}_{j\in[\kTree]}$
        \FOR{$j=1$ to $\kTree$}
            \STATE Set
            \[
            \estSOO_{h+1,j}
            \leftarrow
            \estSOO_{h+1,j}\!\left(\lfloor \hmax/(hm)\rfloor\right),
            \qquad
            \num_{h+1,j}
            \leftarrow
            \lfloor \hmax/(hm)\rfloor.
            \]
        \ENDFOR
    \ENDFOR
\ENDFOR

\vspace{0.4em}
\STATE \textcolor{blue}{\%\textsf{Re-evaluation phase}}
\FOR{$p=0$ to $\lfloor \log_2(\hmax)\rfloor$}
    \STATE Select
    \[
    (h_p,i_p)\in
    \arg\max_{(h,i)\in \tree\,:\,\num_{h,i}\ge 2^p}
    \estSOO_{h,i}.
    \]
    \STATE Re-evaluate:
    \[
    \estSOO_{h_p,i_p}
    \leftarrow
    \estSOO_{h_p,i_p}\!\left(\lfloor \hmax/2\rfloor\right).
    \]
\ENDFOR

\STATE Set
\[
\pOut \leftarrow \arg\max_{p\in[\lfloor\log_2(\hmax)\rfloor]} \estSOO_{h_p,i_p},
\quad
\returnSol \leftarrow \varSOO_{h_{\pOut},i_{\pOut}},
\quad
\returnVal \leftarrow \estSOO_{h_{\pOut},i_{\pOut}}.
\]

\RETURN $\returnVal,\returnSol$
\end{algorithmic}
\end{algorithm}
