# Supplementary material for: EXOTIC: An Exact, Optimistic, Tree-Based Algorithm for Min-Max Optimization
Source: arXiv:2508.12479 source file (2026-05-23)
Supplement: Supplementary file 3 [file Gradient_Descent_Convergence.tex]

% Suppose, we want to solve the following optimization problem: 
% \begin{align*}
%     \min_{x\in X} f(x),
% \end{align*}
% where \(X\) is a convex, compact set, and \(f: X \rightarrow \mathbb{R}\) is a convex function. Furthermore,
% Let \(x^\ast\) be the optimal solution. That is, \(x^\ast \in \arg\min_{x\in X} f(x)\). 

% The projected gradient descent algorithm can be formulated as follows 
% \begin{align*}
%     x_{t+1} = \Pi_{X} (x_{t} - \eta \nabla f(x)), 
% \end{align*}
% where \(\Pi_X\) is the projection operator. 

% \begin{theorem}\label{thm: ConvGAProof}
%     If \(\eta \in (0, 1/\beta],\) then 
%     \begin{align*}
%         \min_{t\in[T]}f(x_{t})-f(x^\ast) \leq \frac{1}{2 T \eta}\|x_0-x^\ast\|^2.
%     \end{align*}
% \end{theorem}


% \begin{proof}
%     Define an update \(\{y_t\}_{t=1}^{T}\) such that 
%     \begin{align*}
%         y_{t+1} = x_{t} - \eta \nabla f(x_t).
%     \end{align*}
%     Consequently, we have \(x_{t+1} = \Pi_X(y_{t+1})\). 

%     First, we use the \(\beta\)-smoothness property of function to ensure that 
%     \begin{align}\label{eq: Cond11}
%         f(x_{t+1}) \leq f(x_t) + \nabla f(x_t)^\top (x_{t+1}-x_t)+ \frac{\beta}{2}\|x_{t+1}-x_t\|^2.
%     \end{align}

    
%     Next, we note that \(\langle x_{t+1} - y_{t+1}, x_{t+1} - x^\ast  \rangle \leq 0 \). This can be derived from the first order conditions of optimality of the projection operator. Using \(y_{t+1} = x_t - \eta \nabla f(x_t)\), we obtain 
%     \begin{align*}
%         (x_{t+1} - (x_t-\eta \nabla f(x_t)))^{\top}(x_{t+1}-x^\ast)\leq 0. 
%     \end{align*}
%     Rearranging the above terms, we obtain 
%     \begin{align}\label{eq: Cond2}
%         \nabla f(x_t)^\top (x_{t+1}-x^\ast) \leq \frac{1}{\eta}(x_t- x_{t+1})^\top(x_{t+1}-x^\ast)
%     \end{align}

%     Furthermore, from the convexity of \(f\), we know that 
%     \begin{align*}
%         f(x^\ast) \geq f(x_t) + \nabla f(x_t)^\top (x^\ast - x_t),
%     \end{align*}
%     which, upon rearranging, gives us 
%     \begin{align}\label{eq: Cond3}
%         \nabla f(x_t)^\top (x^\ast-x_t) \leq f(x^\ast) - f(x_t).
%     \end{align}

%     Adding \eqref{eq: Cond2} and \eqref{eq: Cond3}, we obtain 
%     \begin{align*}
%        f(x_t) - f(x^\ast)   \leq \nabla f(x_t)^{\top}(x_{t}-x_{t+1})  + \frac{1}{\eta}(x_t- x_{t+1})^\top(x_{t+1}-x^\ast)
%     \end{align*}

%     Finally, noting that 
%     \begin{align*}
%         (x_t-x_{t+1})^{\top} (x_{t+1}-x^\ast) = \frac{1}{2}\left( \|x_t-x^\ast\|^2 - \|x_{t+1}-x^\ast\|^2 - \|x_{t}-x_{t+1}\|^2 \right)
%     \end{align*}

% We obtain 
% \begin{align*}
%     \nabla f(x_t)^{\top}(x_{t+1}-x_{t}) \leq  f(x^\ast) - f(x_t)   + \frac{1}{2\eta} \left(\|x_t-x^\ast\|^2 - \|x_{t+1}-x^\ast\|^2 - \|x_{t}-x_{t+1}\|^2  \right)
% \end{align*}

% Combining this with \eqref{eq: Cond11}, we obtain

% \begin{align*}
%     f(x_{t+1})-f(x^\ast) &\leq  \frac{1}{2\eta} \left(\|x_t-x^\ast\|^2 - \|x_{t+1}-x^\ast\|^2 - \|x_{t}-x_{t+1}\|^2  \right) + \frac{\beta}{2}\|x_{t}-x_{t+1}\|^2 \\ 
%     &\leq  \frac{1}{2\eta} \left(\|x_t-x^\ast\|^2 - \|x_{t+1}-x^\ast\|^2\right) + \left(\frac{\beta}{2}- \frac{1}{2\eta}\right)\|x_{t}-x_{t+1}\|^2
% \end{align*}

% Since \(\eta \leq (1/\beta)\), the last term can be dropped. Therefore, 
% \begin{align*}
%     f(x_{t+1})-f(x^\ast) \leq \frac{1}{2\eta} \left(\|x_t-x^\ast\|^2 - \|x_{t+1}-x^\ast\|^2\right) 
% \end{align*}

% Summing this from \(t=0\) to \(T-1\) and dividing by \(T\) we obtain

% \begin{align*}
%     \frac{1}{T}\sum_{t=0}^{T-1}  (f(x_{t+1})-f(x^\ast) ) \leq \frac{1}{2 T \eta}\|x_0-x^\ast\|^2
% \end{align*}

% This implies, 
% \begin{align*}
%     \min_{t\in[T]}f(x_{t})-f(x^\ast) \leq \frac{1}{2 T \eta}\|x_0-x^\ast\|^2.
% \end{align*}
% \end{proof}
