# Supplementary material for: EXOTIC: An Exact, Optimistic, Tree-Based Algorithm for Min-Max Optimization
Source: arXiv:2508.12479 source file (2026-05-23)
Supplement: Supplementary file 4 [file ProofHandcraftMain.tex]

To prove Proposition \ref{prop: HandCraftExample}, we begin by reformulating~\eqref{eq: toy_example} by introducing the aggregate variables \(
    X := \mathbf{1}^\top \mathbf{x},\) \(
    Y := \mathbf{1}^\top \mathbf{y}.\)
Under this transformation, \eqref{eq: toy_example} reduces to the one-dimensional form
\begin{align*}
    \min_{X \in [-c \xSetDim, \; c \xSetDim]} \;
    \max_{Y \in [-\ySetDim, \; \ySetDim]} \;
    \hat{f}(X, Y)
    = -Y^{3} + XY .
\end{align*}
For any fixed \(X \in [-c \xSetDim, c \xSetDim]\), define 
\(    Y^\ast(X) := \underset{Y \in [-\ySetDim, \, \ySetDim]}{\arg\max} \hat{f}(X, Y).
\)
One can verify that \begin{align*} Y^\ast(X) = \begin{cases} -\ySetDim & \text{if } X \in [-c\xSetDim,\, 0.75 \ySetDim^2[, \\ \{-\ySetDim,\, 0.5 \ySetDim\} & \text{if } X = 0.75 \ySetDim^2, \\ \sqrt{X/3} & \text{if } X \in\, ]0.75 \ySetDim^2,\, c\xSetDim[. 
\end{cases} 
\end{align*}
Next, we define the function \(
    \Phi(X) := \max_{Y \in [-\ySetDim, \ySetDim]} \hat{f}(X, Y)
    = \hat{f}(X, Y^\ast(X))\) and
\[
    \Phi(X) =
    \begin{cases}
        \ySetDim^3 - \ySetDim X, & X \in [-c\xSetDim,\, 0.75 \ySetDim^2], \\[0.5ex]
        \tfrac{2}{3\sqrt{3}} X^{3/2}, & X \in \,]0.75 \ySetDim^2,\, c\xSetDim].
    \end{cases}
\]
We note that \(\Phi\) is decreasing on \([-c\xSetDim,\, 0.75\ySetDim^2]\) and increasing on \([0.75\ySetDim^2,\, c\xSetDim]\). Hence its global minimum is attained at \(X = 0.75\ySetDim^2\). This completes the proof.
